# Supplementary material for: Mining higher-order triadic interactions
Source: arXiv:2404.14997 source file (2025-09-30)
Supplement: Supplementary file 1 [file Mining_triadic_interactions_supplementary_material.pdf]

# Supplemental Material on "Mining higher-order triadic interactions"

Anthony Baptista,[1,2] Marta Niedostatek,[1] Jun Yamamoto,[3] Ben MacArthur,[2,4,5]
Jürgen Kurths,[6,7] Ruben Sanchez Garcia,[2,4] and Ginestra Bianconi[1,2]

[1]*School of Mathematical Sciences, Queen Mary University of London, London, E1 4NS, United Kingdom*
[2]*The Alan Turing Institute, The British Library, London, NW1 2DB, United Kingdom*
[3]*Department of Network and Data Science, Central European University, Vienna 1100, Austria*
[4]*School of Mathematical Sciences, University of Southampton, Southampton SO17 1BJ, United Kingdom*
[5]*Faculty of Medicine, University of Southampton, Southampton SO17 1BJ, United Kingdom*
[6]*Potsdam Institute for Climate Impact Research, 14473 Potsdam, Germany*
[7]*Institute of Physics, Humboldt University of Berlin, 12489 Berlin, Germany*

## SUPPLEMENTAL INFORMATION ON THE TRIADIC MODEL WITHIN CONTINUOUS VARIABLES.

We use a network with $N = 10$ nodes $L = 12$ edges and $\hat{L} = 5$ regulatory interactions (shown in Figure 3 of the main text). We consider the time series obtained by integrating the stochastic dynamics of the proposed dynamical model for triadic interactions within continuous variables. The time series is simulated up to a maximum time $t_{max} = 4000$ with a $dt = 10^{-2}$ leading to $4 \times 10^5$ data points. For our analysis we consider the last $200,000$ data points sampled every fifth point leading to $40,000$ time steps. In Figure 2 of the main text we report the analysis done for the triplet [4,9,5], which is triadic. For this figure the parameters of the model are: $\alpha = 0.05, \hat{T} = 10^{-3}, \Gamma = 10^{-2}$, $w^+ = 8, w^- = 0.5$, number of bins $P = 400$. In the Supplemental Figures S1 and S2 we report the analysis conducted on the same triadic triple of nodes for different parameter values: for Figure S1 we have $\alpha = 0.01, \Gamma = 10^{-2}$, for Figure S2 we have $\alpha = 0.05, \Gamma = 5 \times 10^{-2}$. The other parameter values are the same as in Figure 2 of the main text.

## SUPPLEMENTAL INFORMATION ON ANALYSIS OF GENE-EXPRESSION DATASET

### Triplet selection

We choose two sub-samples of 5000 triples of triadic interactions from the gene-expression associated with Acute Myeloid Leukemia (AML) dataset for our Triaction analyses. The selection process for these sub-samples is motivated by studies indicating that for gene expression data, most of the genes involved in trigenic processes are also involved in digenic processes [1]. Hence, we utilize the Protein-Protein Interaction network (PPI) associated with AML, which captures digenic processes, to choose edges forming the triplets in our study. The selection of the regulatory node aims to encompass both short-range and longer-range interactions. To differentiate between these cases, we employ the shortest path distance in the PPI. The first sub-sample comprises short-range motifs, including the fully connected triangle and the partially connected triangle (see Figure S3(a)). We conduct a similar analysis for longer-range interactions. Figure S3(a) illustrates the distribution of the proportion of triplets categorized by the length of the shortest path between node Z and the edge composed of nodes X and Y. This path length can be expressed as $\min(d_{XZ}, d_{YZ})$, where $d_{XZ}$ denotes the shortest path length between nodes X and Z, and $d_{YZ}$ indicates the shortest path length between nodes Y and Z.

### Comparison between short-range and longer range triples in AML dataset

Based on the structural network, specifically the Protein-Protein Interaction network (PPI), we distinguish interactions into short-range (depicted in blue) and longer-range (depicted in red). Longer-range interactions are characterised by a minimum shortest path between structural edges and the regulatory node candidate of at least 2. S3(b) display the probability density function estimated by Gaussian kernels on the histogram of the probability distribution of the score $\Theta$ for the three measures: $\Sigma$, $T$, and $Tn$. Curves in varying shades of blue represent short-range interactions, while those in shades of red represent longer-range interactions. Notably, significant $\Theta$ scores are predominantly associated with short-range interactions. S3(e-f) showcase correlations between $\Theta$ scores for the three measures. There is a strong correlation between $\Theta_\Sigma$ and $\Theta_T$ (S3(e)), these correlation is observed both for short- and long-range interactions. The correlation is also observed between $\Theta_\Sigma$ and $\Theta_{T_n}$ ((S3(f))). S3(c-d) display mutual information between nodes ($X$ and $Y$) involved in structural edges, as well as mutual information between $X$ and

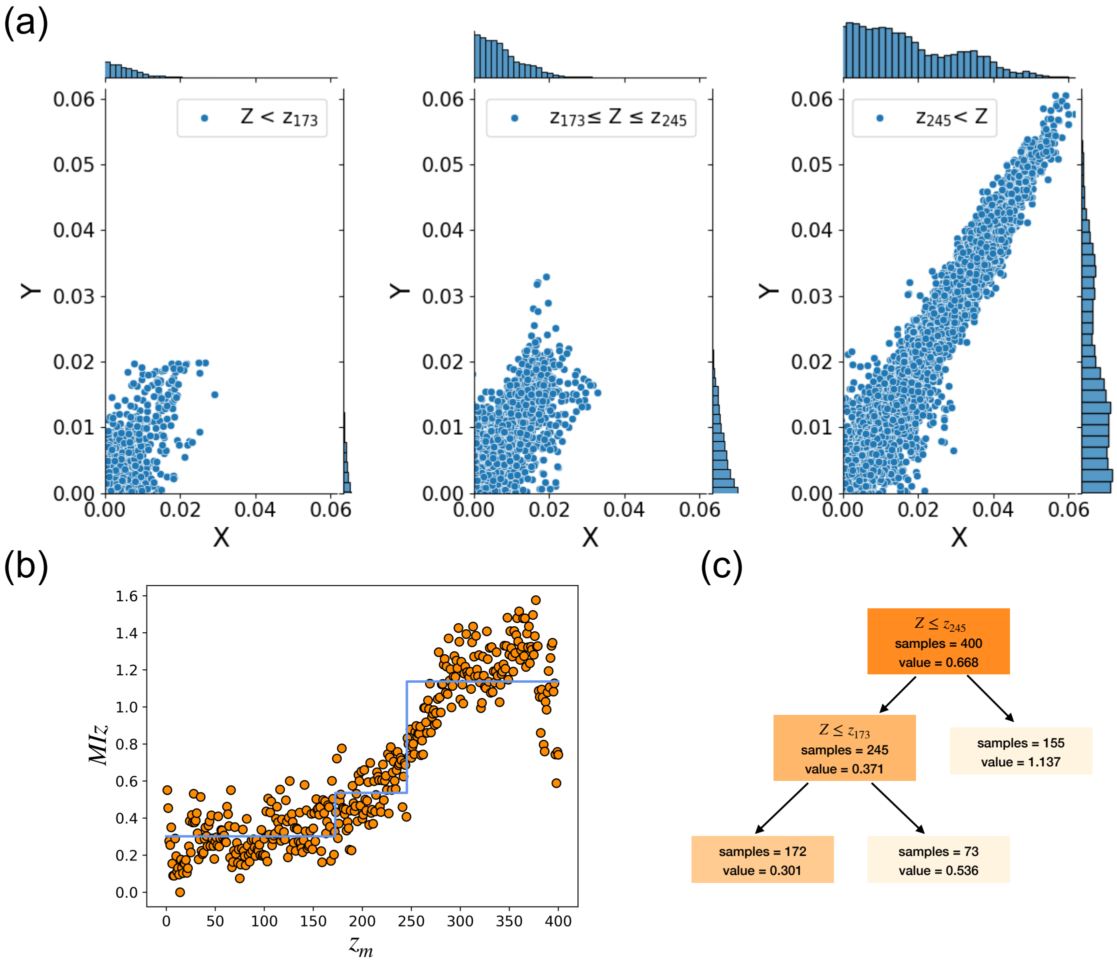


FIG. S1: Exemplary results obtained for a triple of nodes involved in a triadic interactions in the continuous model with triadic interactions. The joint distributions of variables $X$ and $Y$ conditional on the values of $Z$ is shown in panel (a). Panel (b) displays the functional behavior of $MIz$ as a function of the values of $z_m$ which clearly departs from the constant behavior expected in absence of triadic interactions. Panel (c) presents the decision tree for fitting the $MIz$ functional behavior and determining the range of values of $Z$ for which the most significant differences among the joint distributions of the variables $X$ and $Y$ conditional to $Z$ are observed. For more details about the simulation result we refer to the Supplemental Material. The time series is simulated up to a maximum time $t_{max} = 4000$ with a $dt = 10^{-2}$. For the analysis we consider 40000 time steps. The parameters of the model are: $\alpha = 0.01, \hat{T} = 10^{-3}, \Gamma = 10^{-2}$, $w^+ = 8, w^- = 0.5$, number of bins $P = 400$. The analysis is done for the triplet [4,9,5], of the network in Figure 2 of the main text, which is triadic.

$Y$ conditioned by the third node ($Z$), which is designated as the regulatory node. Colour denotes the logarithm of the inverse of the P-value of the $\Sigma$ measure ($P_\Sigma$), emphasising significant P-values. Red dots represent short-range interactions (S3(c)), while blue dots represent longer-range interactions (S3(d)). Observations indicate that significant triplets, particularly for short-range interactions, necessitate high mutual information and conditional mutual information. However, for longer-range interactions, conditional mutual information must be higher that mutual information.

### Comparison between the results obtained with different measures

In Figure S4 we display the results obtained on the gene-expression AML data by performing an analysis conducted using the $T$ and the $T_n$ measures. We observe that these results correlate with the results obtained using the $\Sigma$ measure reported in Fig.4 of the main text.

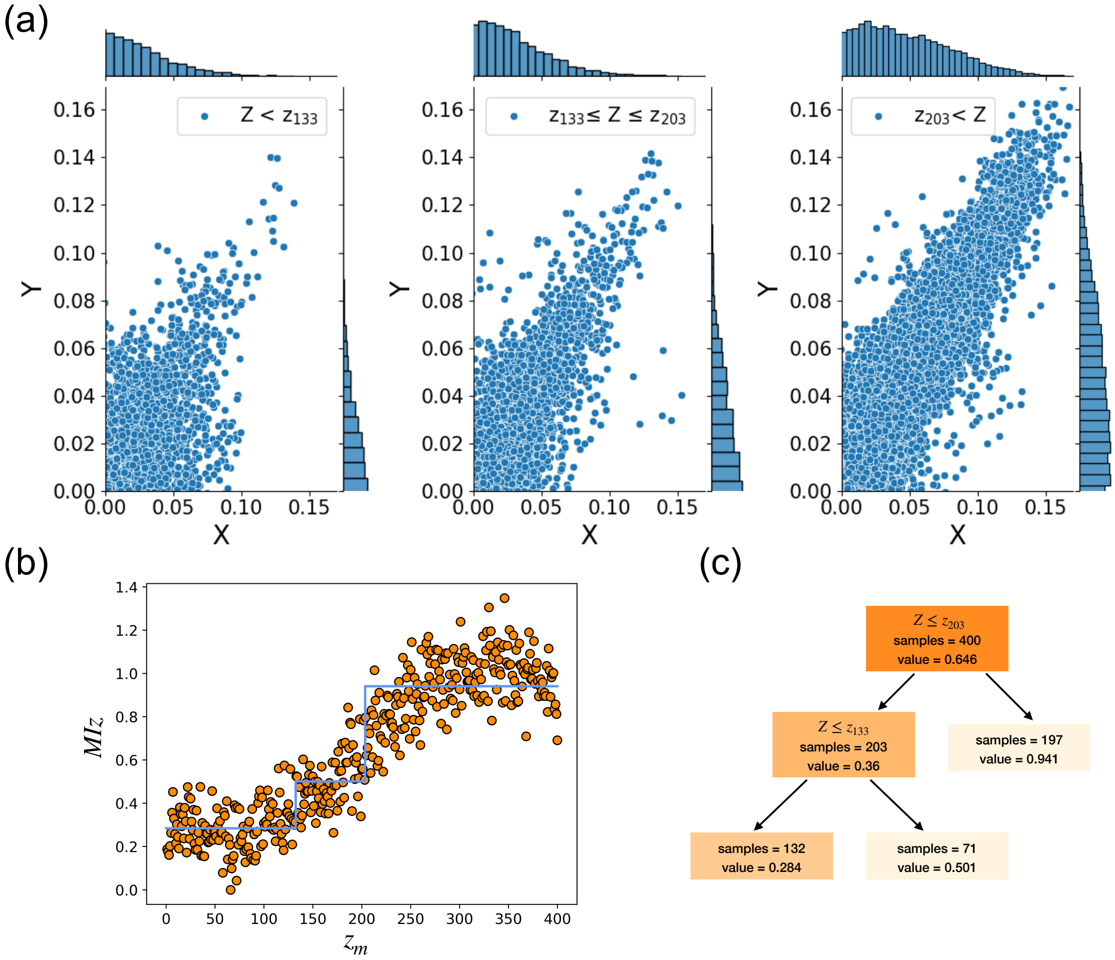


FIG. S2: Exemplary results obtained for a triple of nodes involved in a triadic interactions in the continuous model with triadic interactions. The joint distributions of variables $X$ and $Y$ conditional on the values of $Z$ is shown in panel (a). Panel (b) displays the functional behavior of $MIz$ as a function of the values of $z_m$ which clearly departs from the constant behavior expected in absence of triadic interactions. Panel (c) presents the decision tree for fitting the $MIz$ functional behavior and determining the range of values of $Z$ for which the most significant differences among the joint distributions of the variables $X$ and $Y$ conditional to $Z$ are observed. For more details about the simulation result we refer to the Supplemental Material. The time series is simulated up to a maximum time $t_{max} = 4000$ with a $dt = 10^{-2}$. For the analysis we consider 40000 time steps (see SM for details). The parameters of the model are: $\alpha = 0.05, \hat{T} = 10^{-3}, \Gamma = 5 \times 10^{-2}$, $w^+ = 8, w^- = 0.5$, number of bins $P = 400$.The analysis is done for the triplet [4,9,5], of the network in Figure 2 of the main text, which is triadic.

### Supplemental figure and table of detected triadic interactions in AML dataset

We detected 32 triadic interactions with a $p_\Sigma < 0.001$, listed in Table S1. In the Table, we report $\Sigma, T, T_n$ $\Theta_\Sigma, \Theta_T, \Theta_{T_n}$ and the p-values $p_\Sigma, p_T, p_{T_n}$ associated with each triadic interaction of the network displayed in Figure S5. We observe that the genes involved in the highest triadic interactions regulation are genes to play a critical role in AML (Figure 6), the HOX family [2], PBX3 [3], and MEIS1 [4]. Moreover, a recent study shows that HOXA5 is a regulation hub for AML patients [5] which can also be observed in Figure 6. Furthermore, known triple have been detected with a lower p-value threshold like (HOXA9, PBX3, MEIS1, $p_\Sigma = 0.06$) which are known to cooperate all together in AML patients [6, 7].

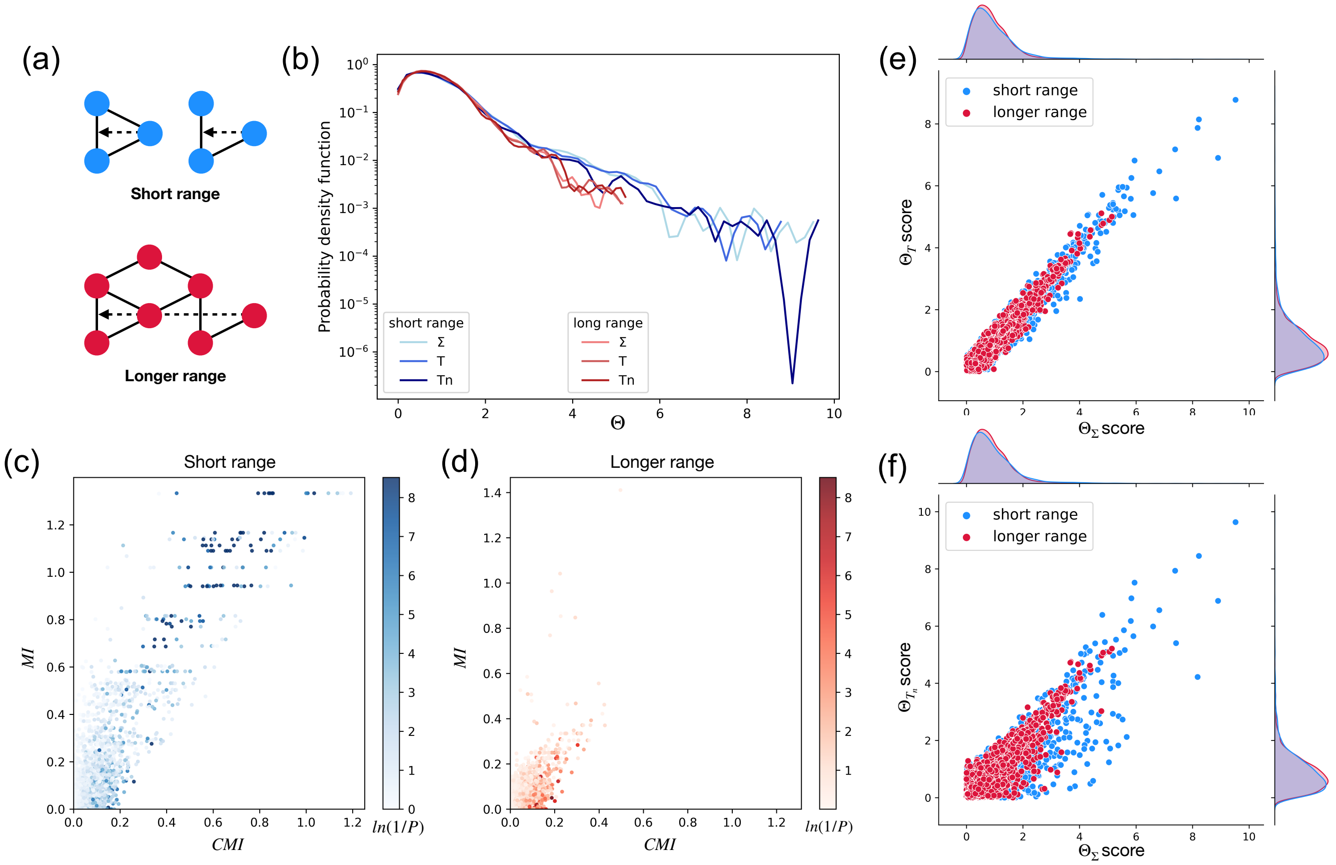


FIG. S3: (a) Candidate triadic interactions occur both at short-range (depicted in blue) and at longer-range (depicted in red). (b) Probability density function of $\Theta$ for the three measures: $\Sigma$, $T$, and $T_n$. Curves in varying shades of blue represent short-range interactions, while those in shades of red represent longer-range interactions. (c-d) Scatter plots of the mutual information between nodes ($X$ and $Y$) involved in structural edges and the mutual information between $X$ and $Y$ conditioned by the third node ($Z$). Color denotes the logarithm of the inverse of the $P$-value of the $\Sigma$ measure ($P_\Sigma$). Red dots represent short-range interactions (c), and blue dots represent longer-range interactions (d). (e-f) Scatter plots between $\Theta$ scores for the three measures: between $\Theta_\Sigma$ and $\Theta_T$ (e), and $\Theta_\Sigma$ and $\Theta_{T_n}$ (f).

### Supplemental Figures on gene-expression results

In Figure S6-S9 we display exemplary results obtained by applying the Triaction algorithm on the AML dataset. Figure *S6* provides an example of high-significant positive triadic interaction. Figure *S6* provides an example of high-significant negative triadic interactions. Figure *S8* provides an example of triadic interactions displaying a non-monotonous $MIz$ functional behavior. Figure *S9* provides an example of triple with low significance score for triadic interactions with a almost flat $MIz$ profile.

## TRIACTION PYTHON PACKAGE

The Triaction algorithm here proposed is implemented by a Python package, called Triaction, that we have developed for detecting triadic interations within continuous and discrete variables. The Triaction package allows to work with both data-frames and data sets associated with a pairwise network. From this initial data, the package provides various ways to extract relevant features and detect triadic interactions. We have included several representations and visualisations in the package to aid in the interpretation of the results. The code is available on GitHub at the following link: https://github.com/anthbapt/triaction. Additionally, we offer documentation to guide users through the analysis process.

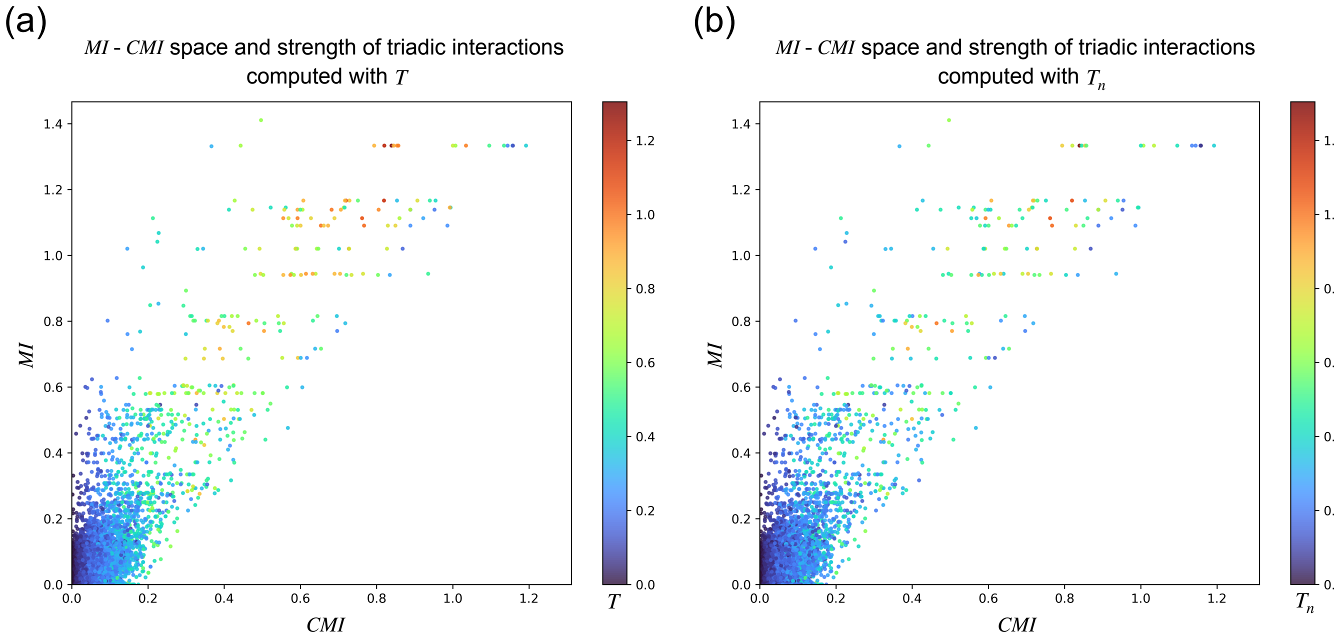


FIG. S4: (a) Scatter plot which displays the MI (Y-axis) value between two genes, denoted $X$ and $Y$, and the CMI (X-axis) between the same genes $X$ and $Y$ conditioned by a third gene, denoted $Z$. The colour corresponds to the value of our measure $T$ which characterises the strength of the triadic interaction between gene $Z$ and edge involving $X$ and $Y$. (b) Same figure for the measure $T_n$.


[1] Elena Kuzmin, Benjamin VanderSluis, Wen Wang, Guihong Tan, Raamesh Deshpande, Yiqun Chen, Matej Usaj, Attila Balint, Mojca Mattiazzi Usaj, Jolanda van Leeuwen, Elizabeth N. Koch, Carles Pons, Andrius J. Dagilis, Michael Pryszlak, Jason Zi Yang Wang, Julia Hanchard, Margot Riggi, Kaicong Xu, Hamed Heydari, Bryan-Joseph San Luis, Ermira Shuteriqi, Hongwei Zhu, Nydia Van Dyk, Sara Sharifpoor, Michael Costanzo, Robbie Loewith, Amy Caudy, Daniel Bolnick, Grant W. Brown, Brenda J. Andrews, Charles Boone, and Chad L. Myers. Systematic analysis of complex genetic interactions. *Science*, 360(6386):eaao1729, April 2018.

[2] R. A. Alharbi, R. Pettengell, H. S. Pandha, and R. Morgan. The role of hox genes in normal hematopoiesis and acute leukemia. *Leukemia*, 27(5):1000–1008, 2013.

[3] Huidong Guo, Yajing Chu, Le Wang, Xing Chen, Yangpeng Chen, Hui Cheng, Lei Zhang, Yuan Zhou, Feng-chun Yang, Tao Cheng, Mingjiang Xu, Xiaobing Zhang, Jianfeng Zhou, and Weiping Yuan. Pbx3 is essential for leukemia stem cell maintenance in mll-rearranged leukemia. *Int. J. Cancer*, 141(2):324–335, July 2017.

[4] Ping Xiang, Xining Yang, Leo Escano, Ishpreet Dhillon, Edith Schneider, Jack Clemans-Gibbon, Wei Wei, Jasper Wong, Simon Xufeng Wang, Derek Tam, Yu Deng, Eric Yung, Gregg B. Morin, Pamela A. Hoodless, Martin Hirst, Aly Karsan, Florian Kuchenbauer, R. Keith Humphries, and Arefeh Rouhi. Elucidating the importance and regulation of key enhancers for human meis1 expression. *Leukemia*, 36(8):1980–1989, 2022.

[5] Huili Wang, Sheng-Yan Lin, Fei-Fei Hu, An-Yuan Guo, and Hui Hu. The expression and regulation of hox genes and membrane proteins among different cytogenetic groups of acute myeloid leukemia. *Molecular genetics & genomic medicine*, 8:e1365, Sep 2020.

[6] Ross M. W. Thorne and Thomas A. Milne. Dangerous liaisons: cooperation between pbx3, meis1 and hoxa9 in leukemia. *haematol*, 100(7):850–853, July 2015.

[7] Zejuan Li, Ping Chen, Rui Su, Chao Hu, Yuanyuan Li, Abdel G. Elkahloun, Zhixiang Zuo, Sandeep Gurbuxani, Stephen Arnovitz, Hengyou Weng, Yungui Wang, Shenglai Li, Hao Huang, Mary Beth Neilly, Gang Greg Wang, Xi Jiang, Paul P. Liu, Jie Jin, and Jianjun Chen. PBX3 and MEIS1 Cooperate in Hematopoietic Cells to Drive Acute Myeloid Leukemias Characterized by a Core Transcriptome of the MLL-Rearranged Disease. *Cancer Research*, 76(3):619–629, 01 2016.

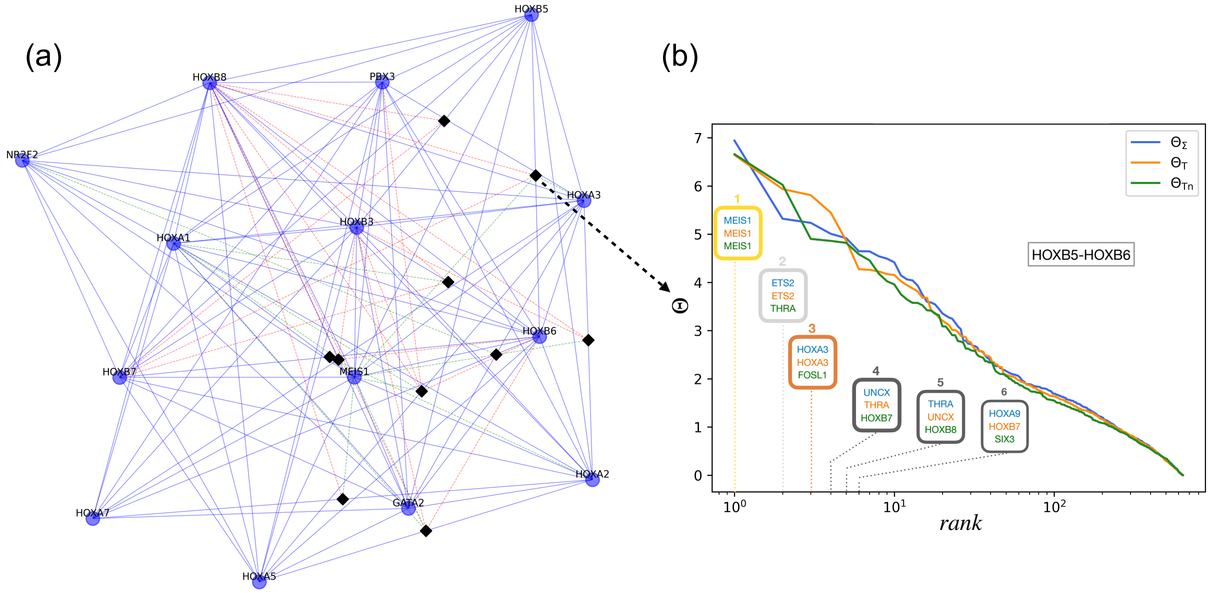


FIG. S5: (a) Visualization of the AML network with triadic interactions mined by the Triaction algorithm including the 32 detected triadic interactions with $p_\Sigma < 10^{-3}$ (see Supplementary Table for the list of such interactions). Blue nodes and edges compose the structural network, which is a subgraph of the Protein-Protein Interaction network (PPI). Factor nodes are depicted as black diamonds, while dashed lines (green for positive and red for negative) illustrate regulatory triadic interactions. (b) We consider all the putative triadic interactions involving the structural network edge HOXB5-HOXB6 and any possible regulatory node. The obtained values of $\Theta_\Sigma$, $\Theta_T$, and $\Theta_{Tn}$, are plotted against their rank. The nodes associated with the six highest ranked $\Theta$ scores are indicated in the insets. Across all three measures ($\Sigma$, $T$, and $Tn$), the top triadic interaction involves MEIS1 as the regulatory node (depicted in a golden frame inset). The second highest regulatory node for the HOXB5-HOXB6 edge is ETS2 for the $\Sigma$ and $T$ measures, and THRA for the $T_n$ measure (illustrated in a silver frame inset). Notably, THRA also ranks highly for the $\Sigma$ measure (ranked 5) and the $T$ measure (ranked 4). The third highest regulatory node for the HOXB5-HOXB6 edge is HOXA3 for both the $\Sigma$ and $T$ measures, and FOSL1 for the $T_n$ measure (highlighted in a bronze frame-inset).

| **Regulator** | **node1** | **node2** | $\Sigma$ | $T$ | $T_n$ | $\Theta_\Sigma$ | $\Theta_T$ | $\Theta_{T_n}$ | $P_\Sigma$ | $P_T$ | $P_{T_n}$ |
|---|---|---|---|---|---|---|---|---|---|---|---|
| HOXB3 | HOXA2 | HOXA5 | 0.280 | 0.870 | 0.518 | 4.310 | 5.070 | 2.437 | 0.0002 | 0.0002 | 0.0164 |
| MEIS1 | HOXA3 | HOXA5 | 0.490 | 1.304 | 1.304 | 9.521 | 8.777 | 9.634 | 0.0002 | 0.0002 | 0.0002 |
| MEIS1 | HOXB5 | HOXB6 | 0.427 | 1.163 | 1.082 | 6.824 | 6.466 | 6.555 | 0.0002 | 0.0002 | 0.0002 |
| HOXB6 | HOXA2 | HOXA5 | 0.292 | 0.835 | 0.530 | 4.727 | 4.861 | 2.598 | 0.0002 | 0.0002 | 0.0130 |
| HOXB8 | HOXA2 | HOXA5 | 0.256 | 0.744 | 0.571 | 3.782 | 4.019 | 3.005 | 0.0002 | 0.0002 | 0.0050 |
| HOXB3 | HOXA2 | HOXA3 | 0.325 | 0.942 | 0.715 | 5.186 | 5.446 | 4.059 | 0.0002 | 0.0002 | 0.0002 |
| PBX3 | HOXA3 | HOXA5 | 0.438 | 1.196 | 0.722 | 8.179 | 7.870 | 4.219 | 0.0002 | 0.0002 | 0.0002 |
| HOXB6 | HOXA3 | HOXA5 | 0.326 | 0.896 | 0.458 | 5.372 | 5.194 | 1.825 | 0.0002 | 0.0002 | 0.0460 |
| HOXB8 | HOXA3 | HOXA5 | 0.329 | 0.981 | 0.694 | 5.372 | 5.862 | 4.003 | 0.0002 | 0.0002 | 0.0004 |
| HOXB6 | HOXA3 | HOXA7 | 0.262 | 0.737 | 0.404 | 4.447 | 4.468 | 1.716 | 0.0002 | 0.0002 | 0.0570 |
| HOXB3 | HOXA3 | HOXA5 | 0.330 | 0.883 | 0.819 | 5.421 | 5.047 | 5.057 | 0.0002 | 0.0002 | 0.0002 |
| HOXB3 | HOXA3 | HOXA7 | 0.291 | 0.820 | 0.528 | 5.180 | 5.232 | 2.931 | 0.0002 | 0.0002 | 0.0074 |
| HOXB7 | HOXB5 | HOXB6 | 0.309 | 0.884 | 0.884 | 4.258 | 4.404 | 5.059 | 0.0002 | 0.0002 | 0.0002 |
| HOXB8 | HOXA3 | HOXA7 | 0.371 | 1.024 | 1.024 | 7.383 | 7.176 | 7.934 | 0.0002 | 0.0002 | 0.0002 |
| HOXA1 | HOXA3 | HOXA5 | 0.411 | 0.948 | 0.854 | 7.416 | 5.589 | 5.402 | 0.0002 | 0.0002 | 0.0002 |
| MEIS1 | HOXA3 | HOXA7 | 0.428 | 1.000 | 0.927 | 8.901 | 6.901 | 6.880 | 0.0002 | 0.0002 | 0.0002 |
| HOXA2 | HOXB6 | HOXB7 | 0.323 | 0.829 | 0.350 | 4.383 | 3.719 | 0.485 | 0.0002 | 0.0014 | 0.2832 |
| HOXA3 | HOXB5 | HOXB6 | 0.358 | 1.074 | 0.624 | 5.386 | 5.950 | 2.849 | 0.0002 | 0.0002 | 0.0062 |
| HOXB8 | HOXA2 | HOXA7 | 0.258 | 0.704 | 0.704 | 3.529 | 3.351 | 3.908 | 0.0006 | 0.0014 | 0.0006 |
| HOXB8 | HOXB3 | HOXB5 | 0.291 | 0.913 | 0.913 | 4.807 | 5.707 | 6.391 | 0.0002 | 0.0002 | 0.0002 |
| HOXA1 | HOXB3 | HOXB6 | 0.254 | 0.715 | 0.715 | 4.076 | 4.118 | 4.722 | 0.0006 | 0.0010 | 0.0002 |
| HOXB7 | HOXB3 | HOXB6 | 0.320 | 0.809 | 0.809 | 5.908 | 5.054 | 5.646 | 0.0002 | 0.0002 | 0.0002 |
| HOXB7 | HOXB3 | HOXB5 | 0.275 | 0.786 | 0.786 | 4.365 | 4.544 | 5.126 | 0.0002 | 0.0002 | 0.0002 |
| MEIS1 | HOXA2 | HOXA3 | 0.343 | 0.916 | 0.839 | 5.603 | 5.177 | 5.161 | 0.0002 | 0.0002 | 0.0002 |
| HOXB8 | HOXA2 | HOXA3 | 0.326 | 0.869 | 0.820 | 5.187 | 4.799 | 4.961 | 0.0002 | 0.0002 | 0.0002 |
| HOXA1 | HOXA3 | HOXA7 | 0.292 | 0.842 | 0.627 | 5.189 | 5.403 | 3.866 | 0.0002 | 0.0002 | 0.0004 |
| HOXB8 | HOXB5 | HOXB6 | 0.296 | 0.872 | 0.872 | 4.051 | 4.394 | 5.032 | 0.0002 | 0.0002 | 0.0002 |
| HOXB8 | HOXB3 | HOXB6 | 0.322 | 0.994 | 0.994 | 5.948 | 6.816 | 7.519 | 0.0002 | 0.0002 | 0.0002 |
| MEIS1 | HOXA2 | HOXA5 | 0.367 | 0.935 | 0.888 | 6.605 | 5.764 | 5.985 | 0.0002 | 0.0002 | 0.0002 |
| HOXA1 | HOXA2 | HOXA5 | 0.256 | 0.665 | 0.548 | 3.732 | 3.283 | 2.765 | 0.0002 | 0.0022 | 0.0102 |
| NR2F2 | GATA2 | HOXA3 | 0.271 | 0.690 | 0.690 | 8.225 | 8.144 | 8.451 | 0.0002 | 0.0002 | 0.0002 |
| MEIS1 | HOXA2 | HOXA7 | 0.266 | 0.664 | 0.632 | 3.780 | 3.049 | 3.276 | 0.0002 | 0.0040 | 0.0042 |

TABLE S1: The list of the 32 high-significant triples involving and new candidates for triadic interactions obtained by applying the Triaction algorithm to the AML gene-expression data.

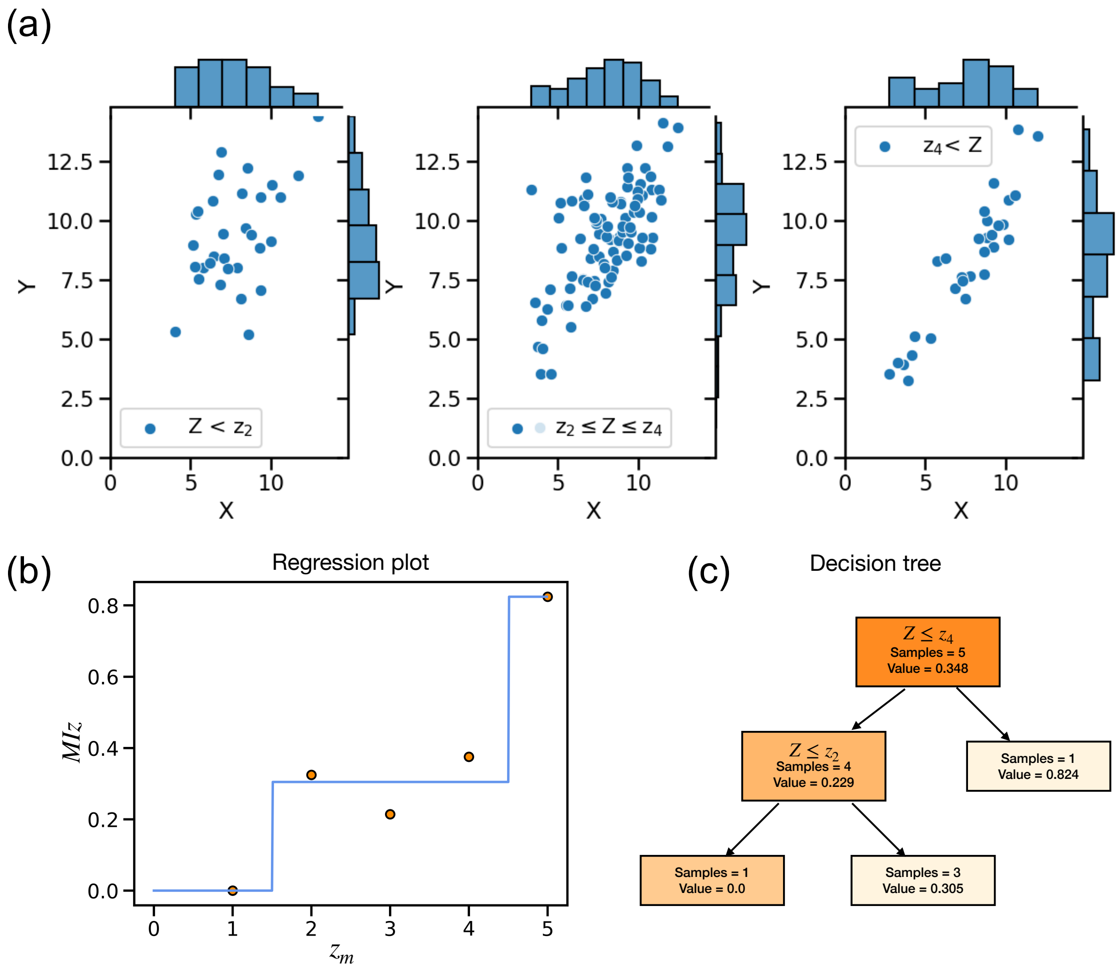


FIG. S6: **Strong triadic interaction:** We choose as thresholds the values defined by the tree to split the data (here $z_2$ and $z_4$). $X$ = GATA1, $Y$ = TAL1, $Z$ = KLF5, $\Sigma = 0.27$, $\Theta_\Sigma = 3.07$, $P_\Sigma = 0.0038$, $T = 0.82$, $\Theta_T = 3.62$, $P_T = 0.0014$, $T_n = 0.45$, $\Theta_{Tn} = 1.19$, $P_{Tn} = 0.124$,, $z_2 = 5.3$, $z_4 = 7.2$

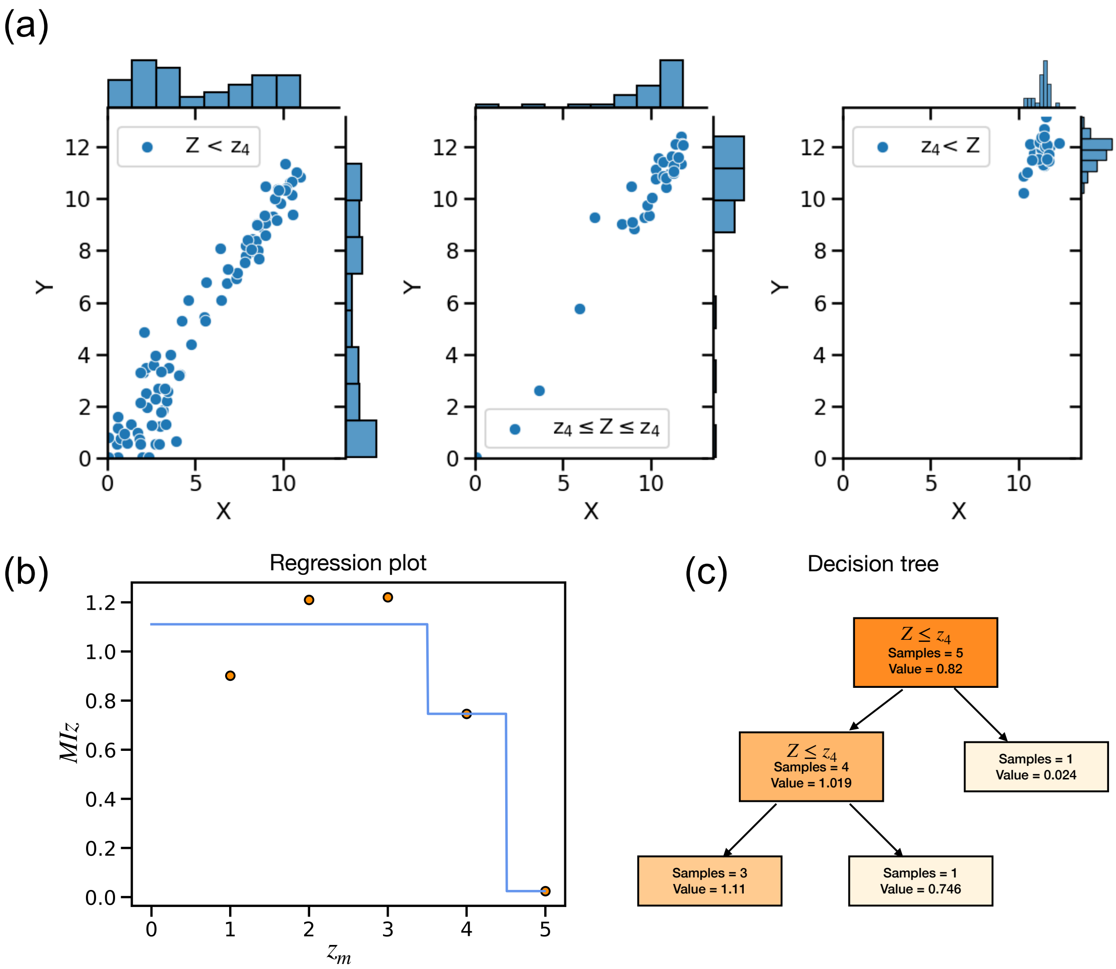


FIG. S7: **Strong triadic interaction:** We choose as threshold the value defined by the tree to split the data ($z_4$). $X$ = HOXA3, $Y$ = HOXA5, $Z$ = PBX3, $\Sigma = 0.44$, $\Theta_\Sigma = 6.33$, $P_\Sigma = 0.0002$, $T = 1.20$, $\Theta_T = 6.07$, $P_T = 0.0002$, $T_n = 0.72$, $\Theta_{Tn} = 3.12$, $P_{Tn} = 0.0048$, $z_4 = 12.8$.

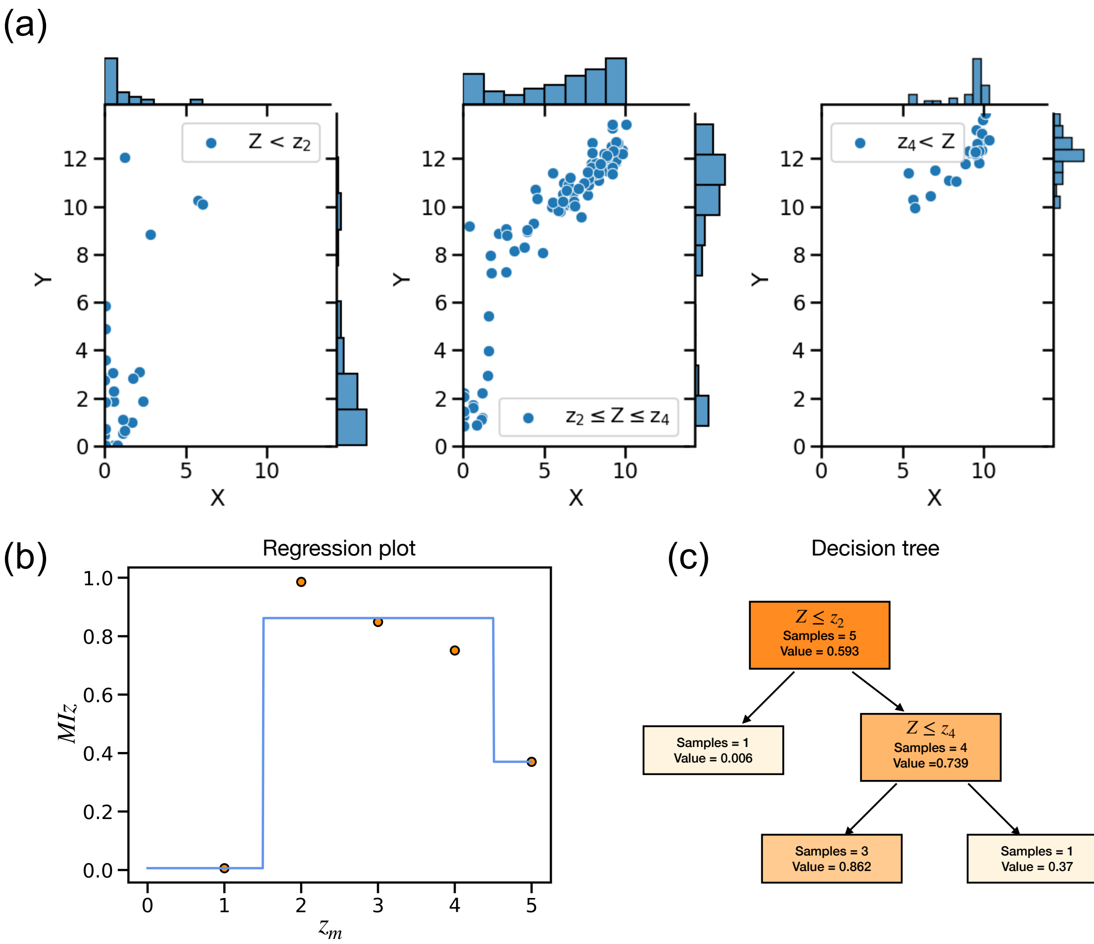


FIG. S8: **Strong triadic interaction:** We choose as thresholds the values defined by the tree to split the data (here $z_2$ and $z_4$). $X$ = HOXA7, $Y$ = HOXA9, $Z$ = HOXA1, $\Sigma = 0.36$, $\Theta_\Sigma = 4.09$, $P_\Sigma = 0.0006$, $T = 0.98$, $\Theta_T = 3.93$, $P_T = 0.0006$, $T_n = 0.98$, $\Theta_{Tn} = 4.52$, $P_{Tn} = 0.0002$,, $z_2 = 4.6$, $z_4 = 7.1$

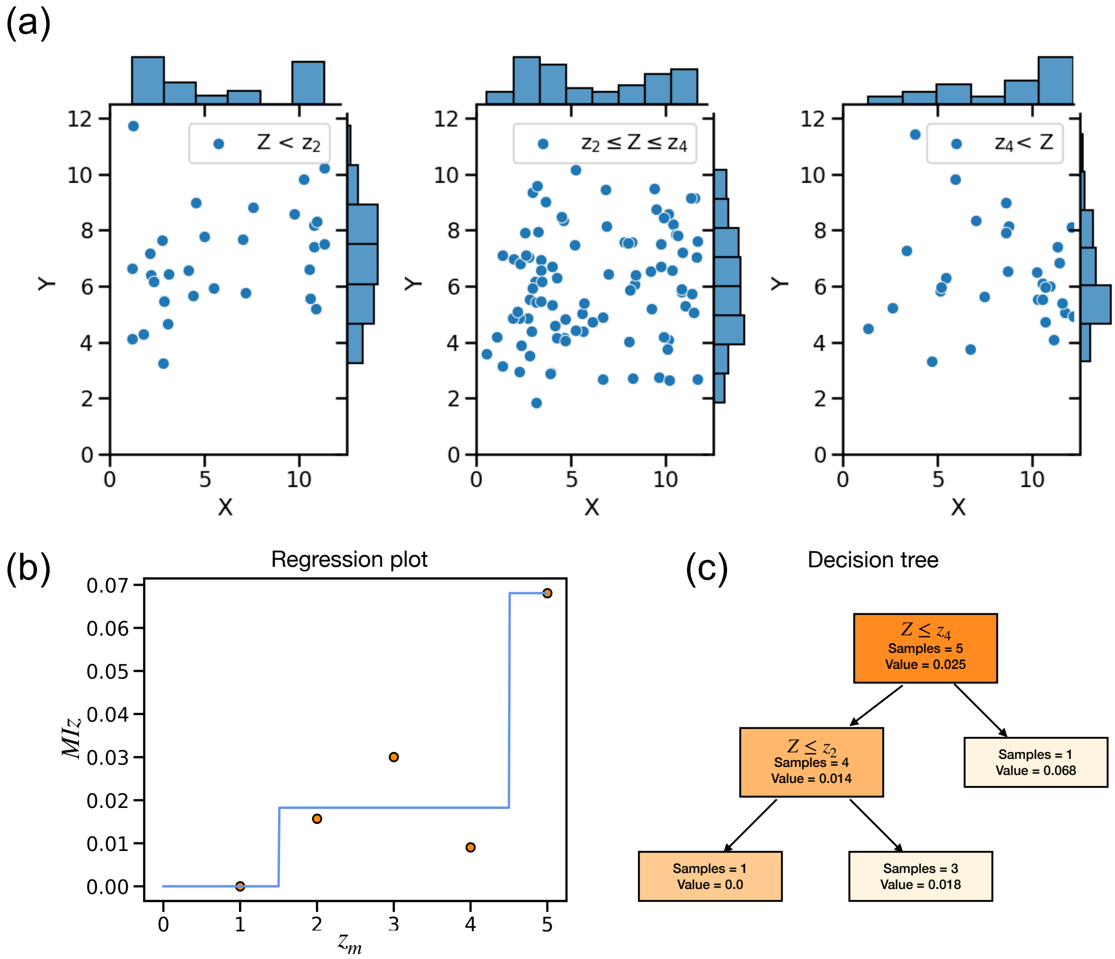


FIG. S9: **Non triadic interaction:** We choose as thresholds the values defined by the tree to split the data (here $z_2$ and $z_4$). $X$ = AR, $Y$ = NR4A3, $Z$ = FLI1, $\Sigma = 0.024$, $\Theta_\Sigma = 0.99$, $p_\Sigma = 0.838$, $T = 0.068$, $\Theta_T = 0.88$, $p_T = 0.81$, $T_n = 0.059$, $\Theta_{Tn} = 0.91$, $P_{Tn} = 0.822$, $z_2 = 12.9$, $z_4 = 13.3$.
